# Supplementary material for: Go with the Flow? A Large-Scale Analysis of Health Care Delivery Networks in the United States Using Hodge Theory
Source: arXiv:2110.09637 source file (2021-12-13)
Supplement: Supplementary file 1 [file supplement.tex]

\beginsupplement

\section{Supporting Information}
